# Supplementary material for: Single particle multipole expansions from Micromagnetic Tomography
Source: arXiv:2101.07010 ancillary file (2021-01-18)
Supplement: Supplementary file 1 [file supp_material.pdf]

# Supplemental Material for ”Single particle multipole expansion from tomography-assisted scanning magnetometry”

David Cortés-Ortuño[1], Karl Fabian[2], and Lennart V. De Groot[1]

[1]Paleomagnetic laboratory Fort Hoofddijk, Department of Earth Sciences, Utrecht University, Budapestlaan 17,, 3584 CD Utrecht, The Netherlands.

[2]Norwegian University of Science and Technology (NTNU), S. P. Andersens veg 15a, 7031 Trondheim, Norway

January 15, 2021

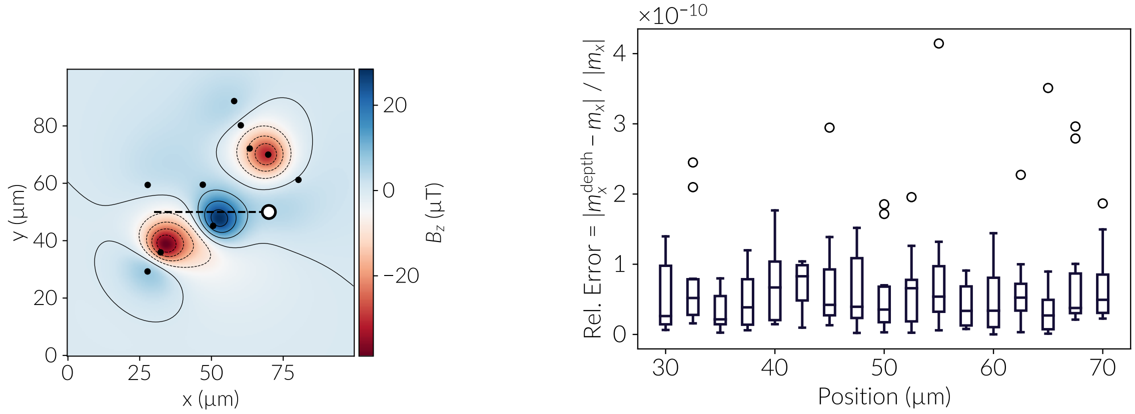


(a) Sample.

(b) Quadrupole inversion results.

SUPP. FIG. S1: Analysis of the inversion of a magnetic sample by shifting the position of a point dipole interacting with other 10 randomly positioned dipole sources with random volumes and dipole moment strength. (a) Overview of the sample where the colormap refers to the scan signal $B_z$ and point sources indicate the positions of the dipole. A straight line indicates the trajectory along which different inversions are performed and analyzed for the dipole (shown as a white dot). (b) Box plot of the inversion result for the shifted particle. The result is shown as the relative error of the $x$-component of the dipole moments. Every box indicates a different point along the trajectory and is the result of 10 inversions with different interacting particles.

# S1 Dipole Inversion Test

The code to invert the signal of point dipoles has been tested with two different approaches. In the first analysis the inversion is tested against the shift of the position of a single particle interacting with 10 other particles. According to this, a sample of $100 \times 100 \times 40$ $\mu$m is defined and 10 point dipoles are randomly positioned and separated by at least 10 $\mu$m distance. These particles are also randomly orientated and generated with volumes in a range between $V = 0.2$ and 1 $\mu$m$^{-3}$, thus their dipole moments are set to $M_s V$ with $M_s = 4.8 \times 10^5$ A/m. Consequently, the particle being

analyzed is positioned at a depth of 20 $\mu$m, at the middle of the sample at $y = 50$ $\mu$m, and oriented in the $(1/\sqrt{3}, 1/\sqrt{3}, 1/\sqrt{3})$ direction with a volume of 1 $\mu$m$^{-3}$. Then starting at $x = 30$ $\mu$m up to 70 $\mu$m, in steps of 2.5 $\mu$m, the sample $B_z$ signal is inverted and the three components of the magnetization are obtained for every position. We repeat this process 10 times with 10 different randomly positioned interacting particles. The arrangement of particles and the corresponding $B_z$ signal for one of these processes is shown in Fig. S1a, where the shifted particle is shown in a white circle with the shifted positions indicated as a line. The result of the inversions is calculated as the relative error of the dipole moments of the shifted particle, for every position. Inversions are performed considering up to the quadrupole order. In Fig. S1b the result of the $x$-component is depicted by a box plot using the 10 samples with randomly generated interacting particles, for every shifted position. Horizontal bars indicate the median of the sample. In this case the $B_z$ signal is noiseless and the relative errors are substantially small, in the order of $10^{-10}$.

In a second test a single particle is also analyzed in a $100 \times 100 \times 40$ $\mu$m sample, and is interacting with 10 other dipolar sources. The magnetic properties of each dipole is set in a similar fashion as in the previous test. The interacting particles are now kept fixed in both position and magnetic properties (volume, orientation) for every run and the particle being analyzed is shifted in position from the top of the sample, starting from 4 $\mu$m, down to 24 $\mu$m depth in steps of 1 $\mu$m. In addition, a Gaussian noise is added to the $B_z$ signal, using a standard deviation in factors of the 2-norm of the $B_z$ array (scan signal). This process is repeated 10 times with different randomly generated noise. The arrangement of particles and the $B_z$ signal

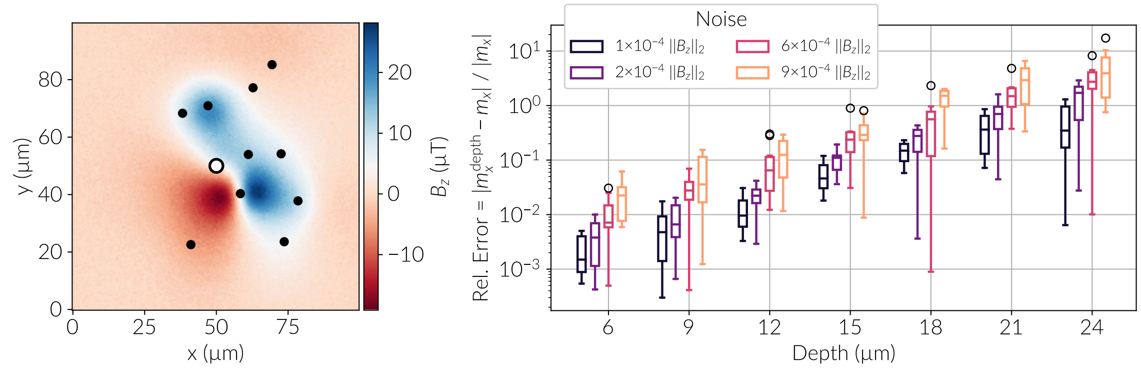


(a) Sample. (b) Quadrupole inversion results.

SUPP. FIG. S2: Analysis of the inversion of a point dipole which is shifted in position across the depth of a sample with 10 interacting particles that are kept with a fixed position. In addition to a change of position, the scan signal is modelled with different noise levels in factors of the 2-norm of the scan signal $B_z$. (a) Overview of the sample with a noise level of $6 \times 10^{-4}||B_z||_2$. Dipole sources are indicated as dots, with the white dot as the particle that is shifted in position. (b) Box plot with the results of the quadrupole inversion of the dipole source at different positions across the sample depth. The results are given as the relative error of the $x$-component of the dipole moment of the shifted particle. Every box is the result of 10 randomly generated Gaussian noise levels with a strength given by a standard deviation in factors of the 2-norm of the scan signal.

is shown in Fig. S2a, with the particle being analyzed in a white circle and using a noise factor of $6 \times 10^{-4}$. Results of the inversion of the $B_z$ signal are computed using a box plot with the 10 different randomly generated noise at selected positions of the particle across the $z$-direction of the sample. In Fig. S2b the results are shown as the relative error of the $x$-component of the dipole moment for 4 different noise strengths and as a function of the depth of the particle in the sample. These calculations are obtained using inversions up to the quadrupole order. With the minimum noise level considered here, the relative errors are always smaller than 0.1 down to a depth

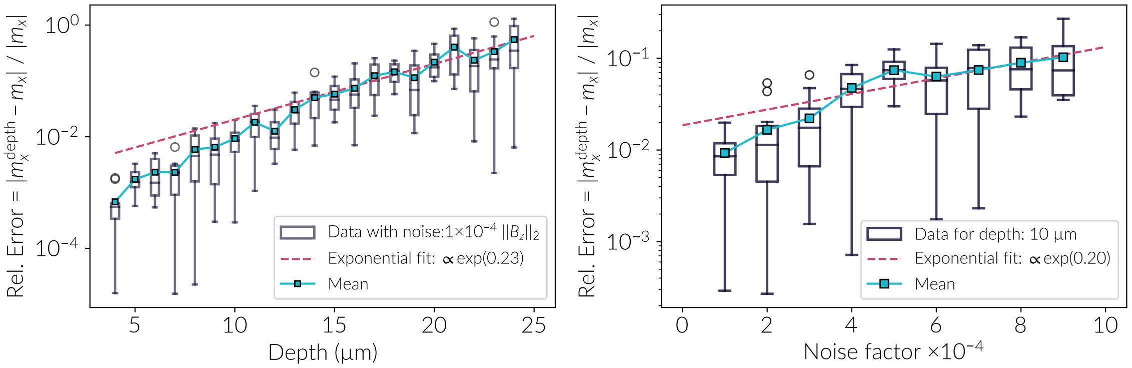


(a) Error against depth.

(b) Error against noise strength.

SUPP. FIG. S3: Least-squares curve fit to the inversion results of a point dipole which is shifted in position across the depth of a sample. (a) An exponential curve fit is shown for the error data as a function of particle depth for a particular noise strength (as a factor of $||B_z||_2$, which is used as the standard deviation of Gaussian noise added to the scan signal $B_z$). Mean values of the errors at every depth are shown with square markers. (b) Similarly than error data of (a) but focusing at a particular particle depth and shown as a function of noise factor (or noise strength).

of approximately 16 $\mu$m. The logarithmic scale of the plot reveals the exponential growth of the errors thus in Fig. S3 exponential curves are fitted to the relative errors for two different cases. In Fig. S3a the relative error for the smallest noise strength, a standard deviation of $1 \times 10^{-4}||B_z||_2$, is shown as a function of particle depth. An exponential least-squares fit $\alpha e^{\beta\, d}$ with $\alpha = 2.03 \times 10^{-3}$, $\beta = 0.23$ and $d$ as the depth in units of micrometer, is shown with a dashed line. The large relative errors for $d > 15\,\mu$m make the curve to fit more optimally in this range of particle depths, which also fits closer to the mean values that are represented as square markers. The same linear tendency is observed for larger noise strengths, where the range of relative error magnitudes increase with increasing noise. According to this, in Fig. S3b the relative errors are computed as a function of noise strength at a particle position of

$10\,\mu$m. Similarly to the first case, an exponential least-squares fit with an exponential factor of $\beta = 0.2$ for noise strength values in orders of $10^{-4}$ optimally describes the growth tendency of the error, in particular for noise factors above $3 \times 10^{-4}$.

# S2 Area 1 Magnetization

The following tables show the numerical data of Fig. 2d-f of the main text, where the magnetization of the grains are obtained for multipole expansions at different orders. These values are compared to those of (de Groot et al., 2018).

| **AREA 1** | **Magnetization A/m** | | | | | | | |
|---|---|---|---|---|---|---|---|---|
| | **Grain** | | | | | | | |
| | 1 | 2 | 3 | 4 | 5 | 6 | 7 | 8 |
| de Groot (2018) | 3544.3 | 3923.7 | 15346.8 | 3770.7 | 28147.8 | 2845.9 | 92191.2 | 7154.4 |
| **Expansion Order** | | | | | | | | |
| Dipole | 3379.87 | 4382.55 | 15254.75 | 4189.07 | 28101.04 | 2130.35 | 88693.4 | 6809.54 |
| Quadrupole | 4611.90 | 6317.08 | 19824.01 | 4272.98 | 39430.48 | 15965.36 | 75775.39 | 14723.43 |
| Octupole | 4488.82 | 8050.03 | 20020.98 | 6485.51 | 24535.00 | 530939.15 | 3637395.37 | 34807.06 |

SUPP. TABLE S1: Magnetization values obtained from inversions in Area 1 of the sample, at different multipole expansion orders. The data presented here corresponds to the data points of Fig. 2d of the main text.

| **AREA 2** | **Magnetization A/m** | | | | | |
|---|---|---|---|---|---|---|
| | **Grain** | | | | | |
| | 1 | 2 | 3 | 4 | 5 | 6 |
| de Groot (2018) | 380.0 | 7309.3 | 18105.1 | 3634.3 | 9700.0 | 7019.7 |
| **Expansion Order** | | | | | | |
| Dipole | 239.76 | 6949.53 | 17948.48 | 3630.84 | 9111.74 | 6760.28 |
| Quadrupole | 1646.46 | 15596.57 | 23319.57 | 6588.19 | 6066.6 | 16428.79 |
| Octupole | 1633.42 | 28900.98 | 27999.54 | 20524.99 | 9044.07 | 77181.34 |

SUPP. TABLE S2: Magnetization values obtained from inversions in Area 2 of the sample, at different multipole expansion orders. The data presented here corresponds to the data points of Fig. 2e of the main text.

| **AREA 3** | **Magnetization A/m** | | | | | |
|---|---|---|---|---|---|---|
| | **Grain** | | | | | |
| | 1 | 2 | 3 | 4 | 5 | 6 |
| de Groot (2018) | 2648.9 | 17527.8 | 5667.3 | 11663.0 | 4285.6 | 8104.8 |
| **Expansion Order** | | | | | | |
| Dipole | 3208.72 | 16740.74 | 5364.76 | 11816.42 | 4014.65 | 7938.28 |
| Quadrupole | 6422.16 | 29592.68 | 5076.97 | 53148.05 | 7854.58 | 58685.14 |
| Octupole | 9871.99 | 42208.73 | 6146.86 | 232150.89 | 25937.98 | 223695.03 |

SUPP. TABLE S3: Magnetization values obtained from inversions in Area 3 of the sample, at different multipole expansion orders. The data presented here corresponds to the data points of Fig. 2f of the main text.

# S3 Multipole Inversion in Area 2 and Area 3

The plots presented here are the result of numerical inversions of the $B_z$ scan signal using different multipole expansion orders, for Area 2 and Area 3 of the sample. In addition, residuals are shown together with the particle positions.

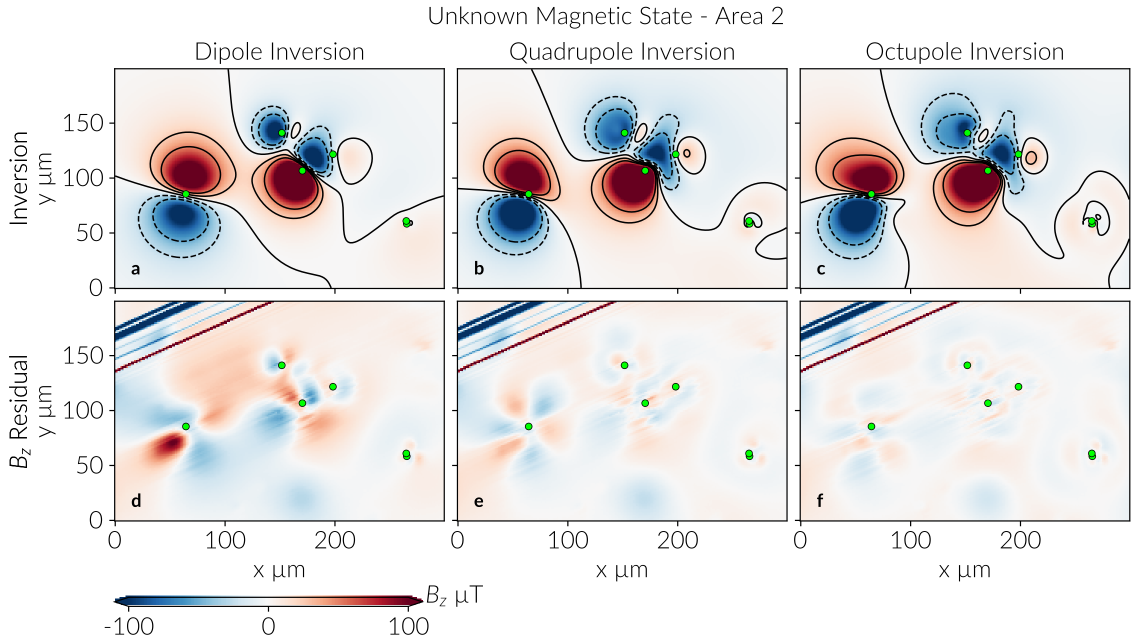


SUPP. FIG. S4: Inversion of area 2 of the SSM scan using multipole expansions at different orders. The sequence of plots shows both the field computed with the inversion and its residual. Contour lines in the field are plotted starting from $-50\,\mu$T up to $50\,\mu$T in steps of $25\,\mu$T. Point magnetic sources (centers of the grains) are plotted as green dots.

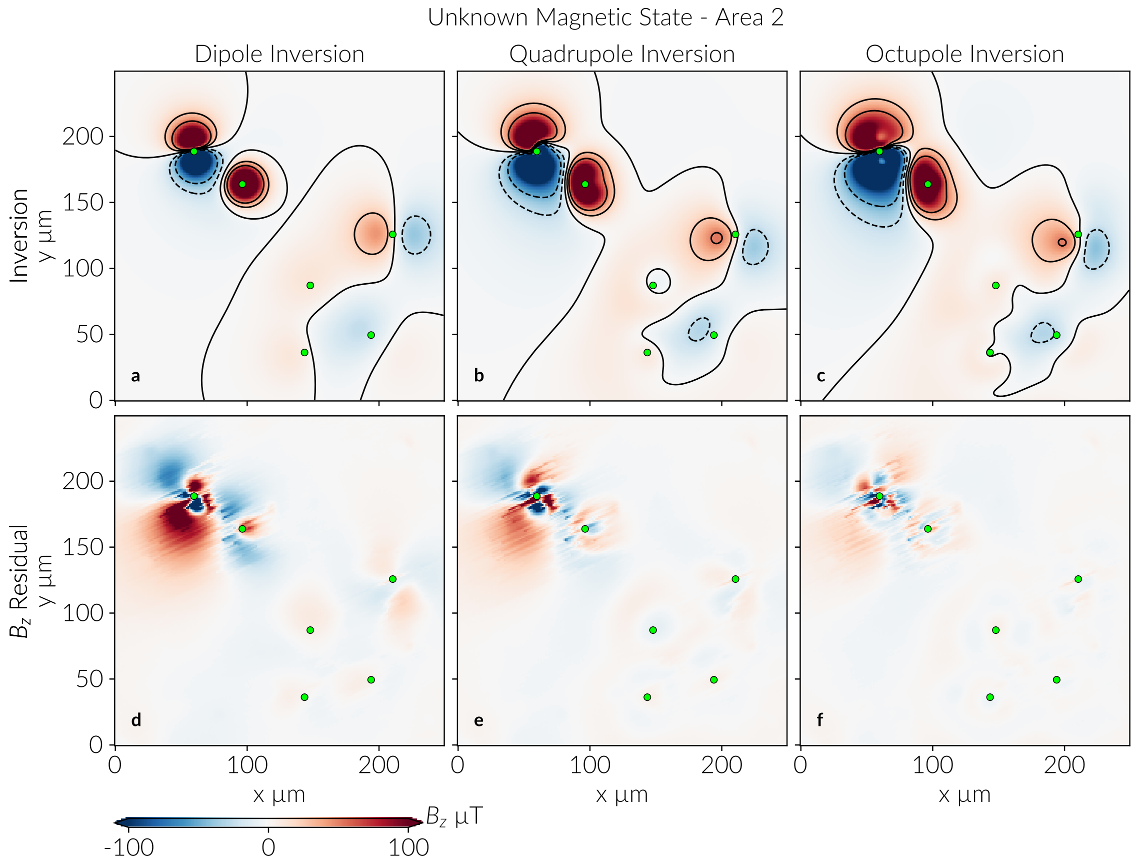


SUPP. FIG. S5: Inversion of area 3 of the SSM scan using multipole expansions at different orders. The sequence of plots shows both the field computed with the inversion and its residual. Contour lines in the field are plotted starting from $-50\,\mu$T up to $50\,\mu$T in steps of $25\,\mu$T. Point magnetic sources (centers of the grains) are plotted as green dots.

# S4 Signal to Noise Ratio

The plots shown here illustrate the regions used to compute the signal-to-noise ratio (SNR) associated to every grain. In every calculation the scan data, a dipole inversion and the residual of this inversion are shown. The regions are computed as rectangular areas covering 90% of the inverted dipole signal, *i.e.* areas surrounding the $B_z$ contour lines with 10% of the maximum dipole signal. Results are shown for the three areas studied in the sample. In the case of Area 2 and Area 3, extra images with the SNR as a function of grain depth are shown. The plots of this section extend the calculations shown in Fig. 3 of the main text.

## S4.1 Area 1

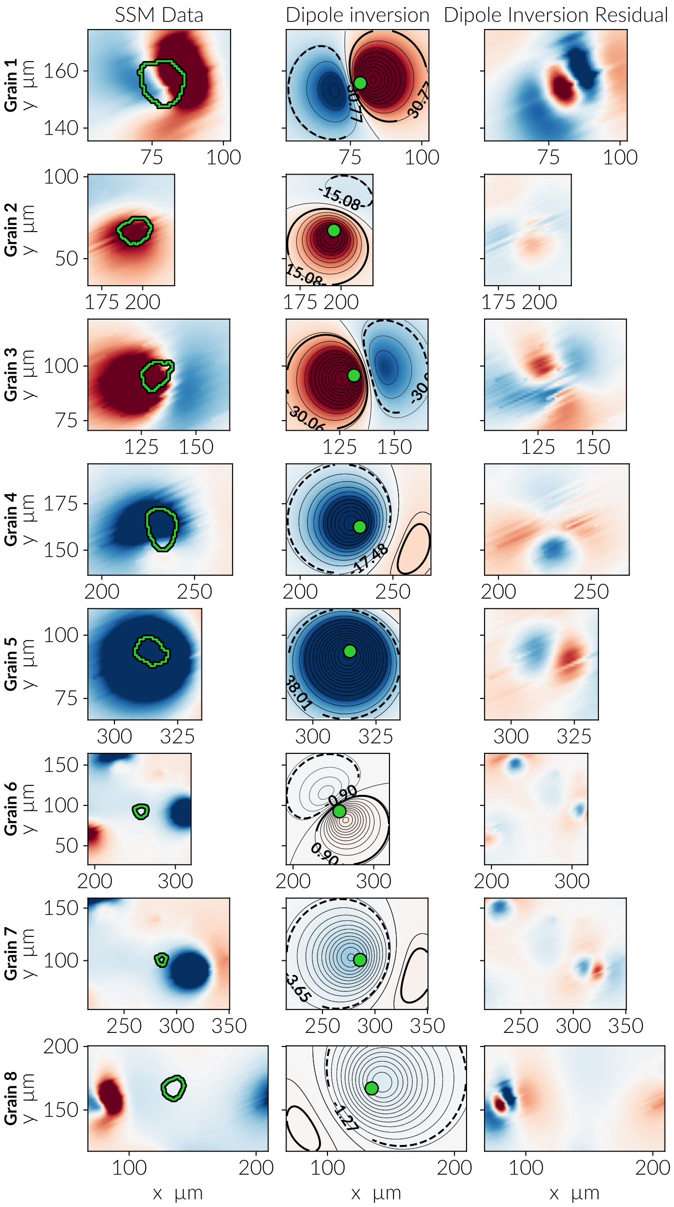


SUPP. FIG. S6: Signal-to-noise ratio calculations in Area 1 of the SSM scan. Every row of plots illustrates details for the calculation of the SNR of the dipolar field generated by a single grain. From left to right, the plots show the original SSM data with the grain boundary, the point dipole model using the dipolar moments from the multipole inversion (up to the dipolar term) and the residual from the inversion. The rectangular areas shown for every case are computed by enclosing the contours containing 90% of the dipole field.

## S4.2 Area 2

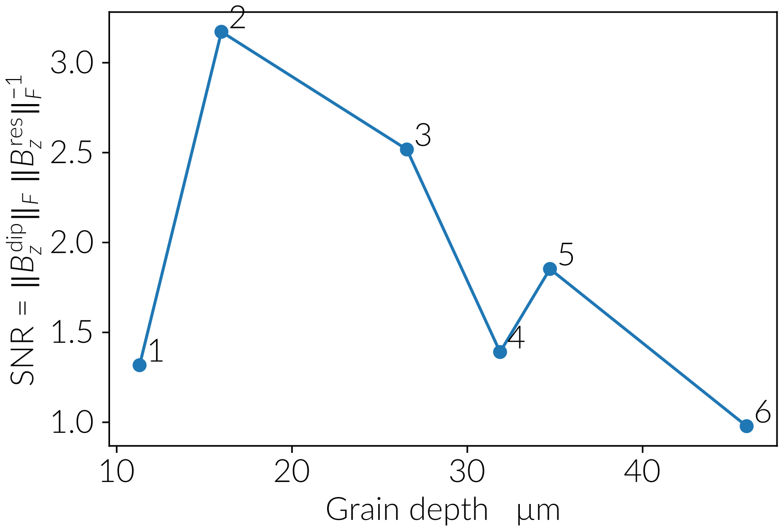


SUPP. FIG. S7: Signal-to-noise ratio as a function of grain depth in Area 2 of the SSM scan. Grain indexes, as specified in the main text, are shown at every data point. Ratios are calculated using the dipole inversions and residuals shown in Fig. S8.

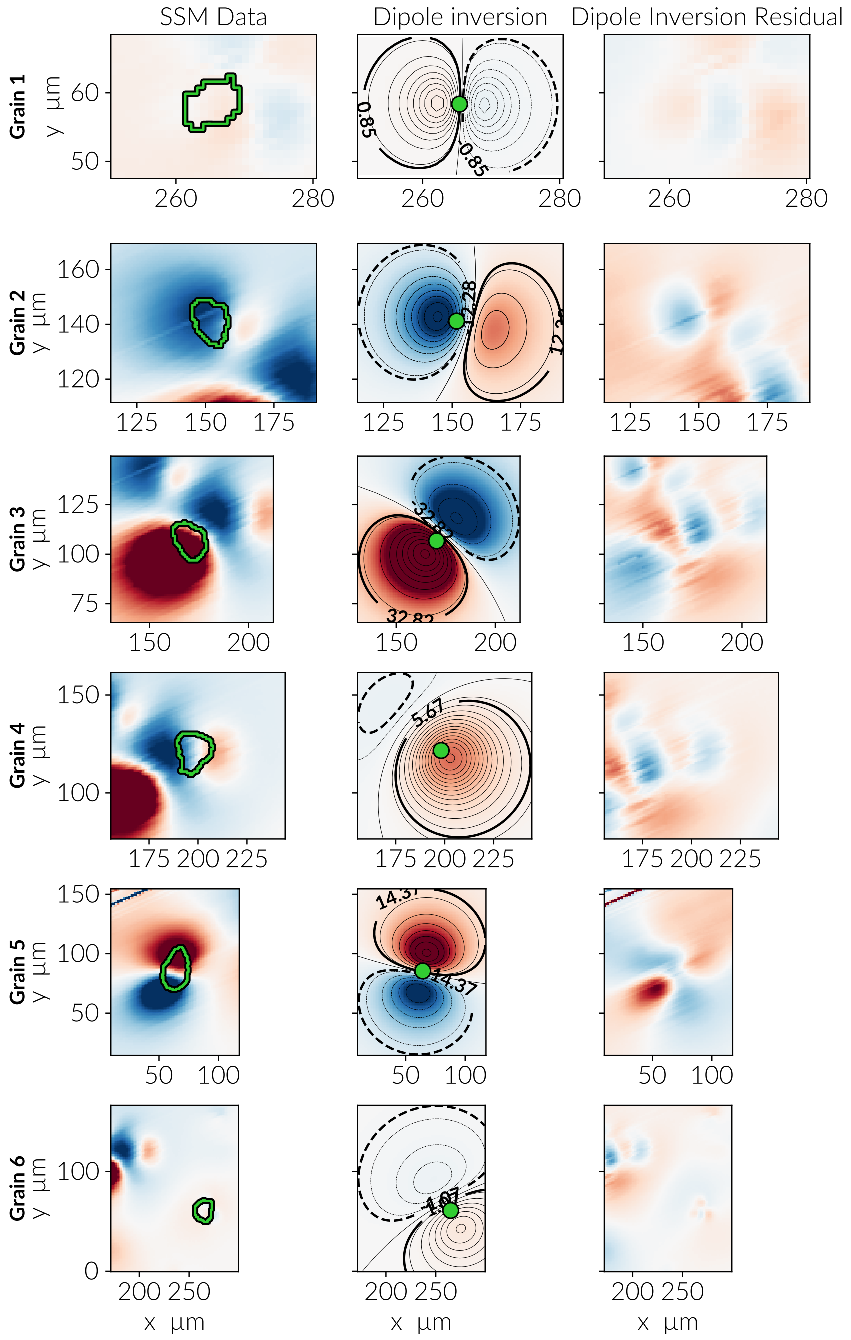


SUPP. FIG. S8: Signal-to-noise ratio calculations in Area 2 of the SSM scan. The sequence of plots are specified in the same fashion as in Fig. S6.

## S4.3 Area 3

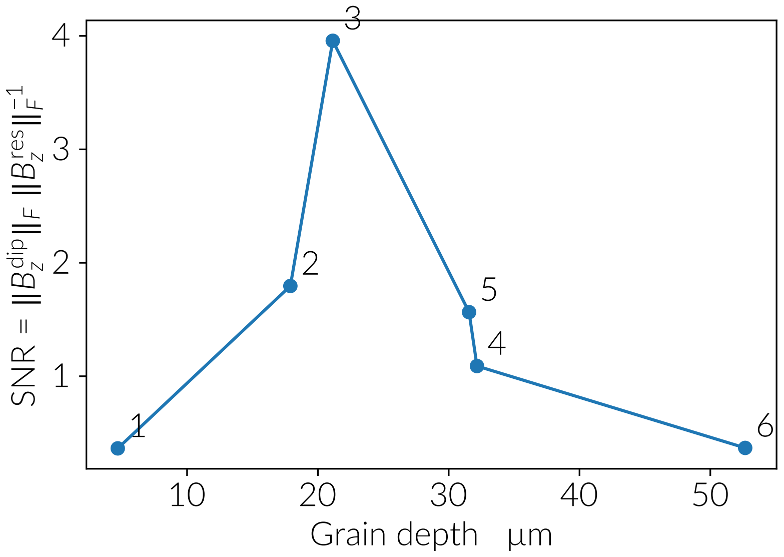


SUPP. FIG. S9: Signal-to-noise ratio as a function of grain depth in Area 3 of the SSM scan. Grain indexes, as specified in the main text, are shown at every data point. Ratios are calculated using the dipole inversions and residuals shown in Fig. S10.

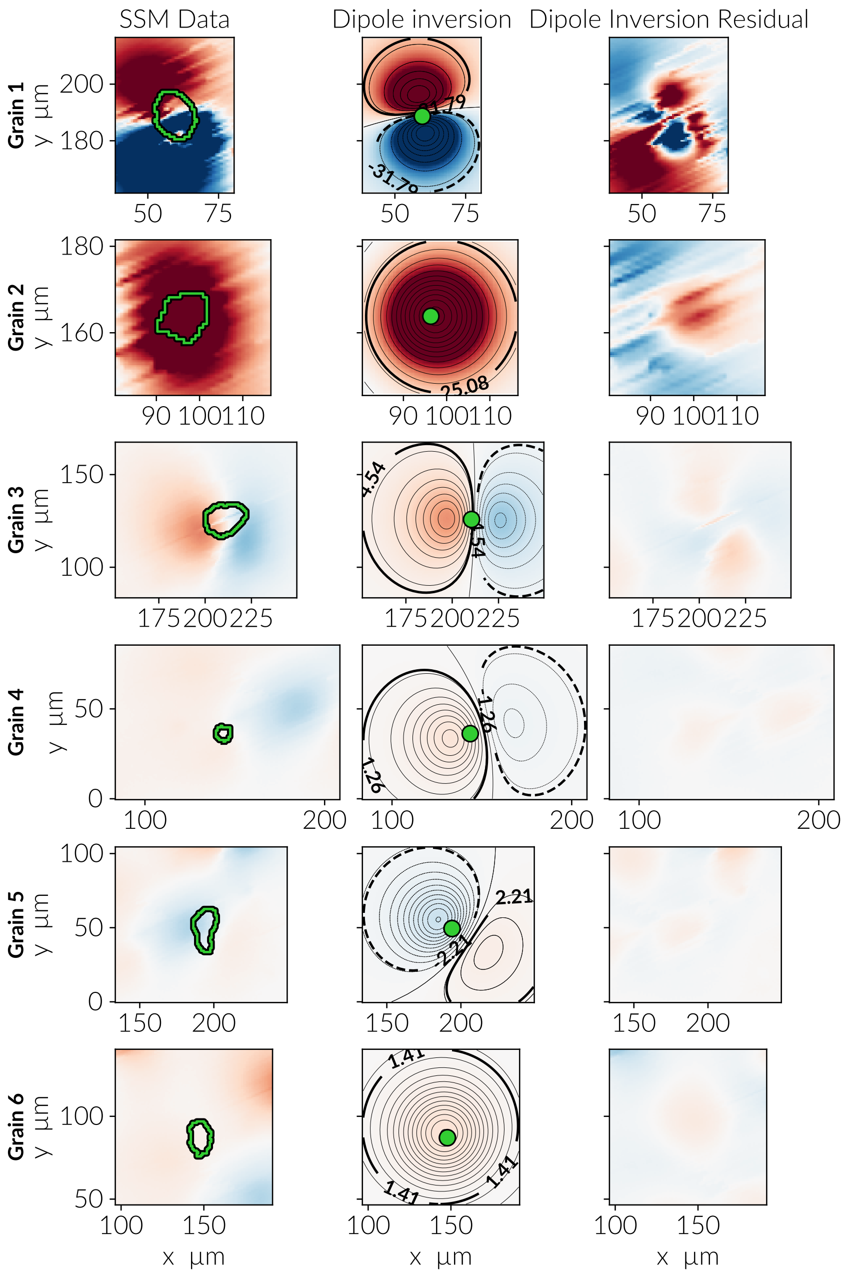


SUPP. FIG. S10: Signal-to-noise ratio calculations in Area 3 of the SSM scan. The sequence of plots are specified in the same fashion as in Fig. S6.

# S5 Inversion results in Area 1

Grain 1

| Order | max(residual) | RMSE | max(signal) |
|---|---|---|---|
| dip | -180.08 µT | 41.53 | 308.48 µT |
| quad | -100.01 µT | 19.61 | 383.35 µT |
| oct | -72.65 µT | 10.84 | 410.40 µT |

Grain 2

| Order | max(residual) | RMSE | max(signal) |
|---|---|---|---|
| dip | -37.24 µT | 12.14 | 148.94 µT |
| quad | 25.38 µT | 6.38 | 120.36 µT |
| oct | -21.70 µT | 4.78 | 134.03 µT |

Grain 3

| Order | max(residual) | RMSE | max(signal) |
|---|---|---|---|
| dip | 77.50 µT | 28.32 | 300.48 µT |
| quad | -59.92 µT | 12.76 | 309.56 µT |
| oct | 65.72 µT | 8.16 | 308.21 µT |

Grain 4

| Order | max(residual) | RMSE | max(signal) |
|---|---|---|---|
| dip | -75.62 µT | 22.05 | -177.95 µT |
| quad | -39.75 µT | 11.56 | -180.31 µT |
| oct | 26.43 µT | 5.74 | -193.93 µT |

Grain 5

| Order | max(residual) | RMSE | max(signal) |
|---|---|---|---|
| dip | 74.97 µT | 19.41 | -379.75 µT |
| quad | -30.77 µT | 5.61 | -377.70 µT |
| oct | -37.85 µT | 4.12 | -372.24 µT |

Grain 6

| Order | max(residual) | RMSE | max(signal) |
|---|---|---|---|
| dip | -15.33 µT | 5.34 | -42.93 µT |
| quad | -8.51 µT | 2.55 | -53.16 µT |
| oct | 7.84 µT | 1.91 | -46.48 µT |

Grain 7

| Order | max(residual) | RMSE | max(signal) |
|---|---|---|---|
| dip | -56.35 µT | 12.78 | -379.75 µT |
| quad | 29.21 µT | 3.90 | -365.06 µT |
| oct | 17.36 µT | 3.35 | -349.89 µT |

Grain 8

| Order | max(residual) | RMSE | max(signal) |
|---|---|---|---|
| dip | 34.11 µT | 10.39 | 15.19 µT |
| quad | 14.85 µT | 4.13 | -24.98 µT |
| oct | 7.07 µT | 2.46 | -21.56 µT |

SUPP. TABLE S4: Output calculations for the residual, inversion and Root Mean Square Error of all grains of Area 1 within a 30 $\mu$m radius around the grain centers. Inversions are performed using multipole expansions at different orders. These values extend those of Table 1 of the main text.

# S6 Inversion results in Area 2

Grain 1

| Order | max(residual) | RMSE | max(signal) |
|---|---|---|---|
| dip | 23.64 µT | 5.81 | 13.40 µT |
| quad | 17.92 µT | 3.96 | 27.26 µT |
| oct | 13.77 µT | 3.30 | 20.07 µT |

Grain 2

| Order | max(residual) | RMSE | max(signal) |
|---|---|---|---|
| dip | -57.56 µT | 18.80 | 144.46 µT |
| quad | 27.14 µT | 7.86 | -107.46 µT |
| oct | -26.44 µT | 5.55 | -108.27 µT |

Grain 3

| Order | max(residual) | RMSE | max(signal) |
|---|---|---|---|
| dip | -65.29 µT | 26.30 | 333.34 µT |
| quad | 40.22 µT | 10.32 | 325.42 µT |
| oct | -27.12 µT | 7.24 | 325.47 µT |

Grain 4

| Order | max(residual) | RMSE | max(signal) |
|---|---|---|---|
| dip | -65.29 µT | 15.61 | 145.58 µT |
| quad | 40.22 µT | 7.88 | 170.92 µT |
| oct | -27.12 µT | 5.19 | 146.72 µT |

Grain 5

| Order | max(residual) | RMSE | max(signal) |
|---|---|---|---|
| dip | 101.65 µT | 34.51 | 143.55 µT |
| quad | -37.13 µT | 18.11 | -179.37 µT |
| oct | -31.08 µT | 9.21 | -187.46 µT |

Grain 6

| Order | max(residual) | RMSE | max(signal) |
|---|---|---|---|
| dip | 23.64 µT | 5.87 | 13.40 µT |
| quad | 17.92 µT | 3.96 | 27.26 µT |
| oct | 13.77 µT | 3.31 | 20.07 µT |

SUPP. TABLE S5: Output calculations for the residual, inversion and Root Mean Square Error of all grains of Area 2 within a 30 $\mu$m radius around the grain centers. Inversions are performed using multipole expansions at different orders. These values extend those of Table 1 of the main text.

## S7 Inversion results in Area 3

Grain 1

| Order | max(residual) | RMSE | max(signal) |
|---|---|---|---|
| dip | -385.04 µT | 68.57 | -324.09 µT |
| quad | -309.38 µT | 49.72 | -266.39 µT |
| oct | 180.67 µT | 30.92 | -255.59 µT |

Grain 2

| Order | max(residual) | RMSE | max(signal) |
|---|---|---|---|
| dip | 97.28 µT | 28.68 | 247.67 µT |
| quad | 88.08 µT | 16.62 | 194.11 µT |
| oct | -82.31 µT | 12.75 | 211.26 µT |

Grain 3

| Order | max(residual) | RMSE | max(signal) |
|---|---|---|---|
| dip | 22.27 µT | 9.03 | 44.54 µT |
| quad | 24.37 µT | 4.54 | 53.27 µT |
| oct | 24.46 µT | 2.86 | 51.75 µT |

Grain 4

| Order | max(residual) | RMSE | max(signal) |
|---|---|---|---|
| dip | 5.96 µT | 2.41 | -18.48 µT |
| quad | 6.28 µT | 1.83 | -21.86 µT |
| oct | -5.39 µT | 1.71 | -22.43 µT |

Grain 5

| Order | max(residual) | RMSE | max(signal) |
|---|---|---|---|
| dip | 6.87 µT | 2.65 | -24.33 µT |
| quad | -6.82 µT | 1.97 | -29.44 µT |
| oct | -5.21 µT | 1.24 | -29.60 µT |

Grain 6

| Order | max(residual) | RMSE | max(signal) |
|---|---|---|---|
| dip | 9.35 µT | 4.13 | 12.59 µT |
| quad | -8.85 µT | 3.64 | 14.92 µT |
| oct | 5.63 µT | 2.15 | 14.14 µT |

SUPP. TABLE S6: Output calculations for the residual, inversion and Root Mean Square Error of all grains of Area 3 within a 30 $\mu$m radius around the grain centers. Inversions are performed using multipole expansions at different orders. These values extend those of Table 1 of the main text.

## S8 Multipole expansion theory

Starting from the definition of the magnetic potential

$$\Phi(\mathbf{R}) = \frac{\mu_0 M_\mathrm{s}}{4\pi} \int_V \frac{\lambda(\mathbf{r})}{|\mathbf{R}-\mathbf{r}|} \mathrm{d}^3 r = \gamma_B \int_V \frac{\lambda(\mathbf{r})}{|\mathbf{R}-\mathbf{r}|} \mathrm{d}^3 r, \tag{1}$$

the standard approach when $|\mathbf{R}| \gg |\mathbf{r}|$ is to expand the coefficient $|\mathbf{R}-\mathbf{r}|^{-1}$. To do this, we notice first that a multidimensional Taylor expansion is expressed as

$$f(\mathbf{x}+\mathbf{a}) \approx f(\mathbf{x}) + \mathbf{a} \cdot \boldsymbol{\nabla} f(\mathbf{x}) + \frac{1}{2!} (\mathbf{a} \cdot \boldsymbol{\nabla}) (\mathbf{a} \cdot \boldsymbol{\nabla}) f(\mathbf{x}) + \ldots$$

In the case of $|\mathbf{R}-\mathbf{r}|^{-1}$, we set $f(\mathbf{x}) = |\mathbf{x}|^{-1}$ and $\mathbf{a} = -\mathbf{r}$ to obtain

$$\frac{1}{|\mathbf{R}-\mathbf{r}|} \approx \frac{1}{|\mathbf{R}|} - r_i \frac{\partial}{\partial R_i} \frac{1}{|\mathbf{R}|} + \frac{1}{2} r_i r_j \frac{\partial^2}{\partial R_i \partial R_j} \frac{1}{|\mathbf{R}|} + \ldots$$

where repeated indices follow Einstein's summation convention. We can summarise this equation in tensor notation as

$$\frac{1}{|\mathbf{R}-\mathbf{r}|} \approx \sum_{n=0}^{\infty} \frac{(-1)^n}{n!} \mathbf{r}^{(n)}_{i_1 i_2 \cdots i_n} \boldsymbol{\nabla}^{(n)}_{i_1 i_2 \cdots i_n} \left(\frac{1}{R}\right), \tag{2}$$

where we have introduced the tensor of magnetic charge positions $\mathbf{r}^{(n)}$ with components

$$\mathbf{r}^{(n)}_{i_1 i_2 \cdots i_n} = r_{i_1} r_{i_2} \cdots r_{i_n},$$

and the tensor $\boldsymbol{\nabla}^{(n)}$ with components

$$\boldsymbol{\nabla}^{(n)}_{i_1 i_2 \cdots i_n} \frac{1}{R} = \frac{\partial^{(n)}}{\partial R_{i_1} \partial R_{i_2} \cdots \partial R_{i_n}} \left(\frac{1}{R}\right).$$

The $\boldsymbol{\nabla}^{(n)}$ tensor is completely symmetric and traceless because $\partial_{ii} R^{-1} = 0$ when $R > 0$. Then the potential is defined as

$$\begin{aligned} \Phi(\mathbf{R}) =& \gamma_B \sum_{n=0}^{\infty} (-1)^n \left[\frac{1}{n!} \int_V \mathrm{d}^3 r \ \lambda(\mathbf{r}) \ \mathbf{r}^{(n)}_{i_1 i_2 \cdots i_n}\right] \boldsymbol{\nabla}^{(n)}_{i_1 i_2 \cdots i_n} \left(\frac{1}{R}\right) \\ =& \gamma_B \sum_{n=0}^{\infty} (-1)^n \, \mathbf{M}^{(n)}_{i_1 i_2 \cdots i_n} \boldsymbol{\nabla}^{(n)}_{i_1 i_2 \cdots i_n} \left(\frac{1}{R}\right), \end{aligned} \tag{3}$$

where $\mathbf{M}^{(n)}$ is the completely symmetric *magnetic moment multipole tensor* of rank $n$, whose components are given as in Equation (3). Following the notation of Burnham & English (2019), we can write the potential using the *inner product of two tensors* $\langle \cdot, \cdot \rangle_t$ as

$$\Phi(\mathbf{R}) = \gamma_B \sum_{n=0}^{\infty} (-1)^n \, \langle \mathbf{M}^{(n)}, \boldsymbol{\nabla}^{(n)} \rangle_t \left(\frac{1}{R}\right). \tag{4}$$

Observe that the term with $n = 0$ refers to a magnetic monopole, which is zero because the total magnetic charge integrates to zero.

It is now necessary to introduce the $\mathbf{R}^{(n)}$ tensors defined as

$$\mathbf{R}^{(n)} = R^{(n)}_{i_1 i_2 \cdots i_n} = R_{i_1} R_{i_2} \cdots R_{i_n},$$

with $\mathbf{R}^{(0)} = 1$ by convention. Applequist (2002) and Burnham & English (2019) discuss that the $\mathbf{R}^{(n)}$ tensors can be projected onto the *subspace of traceless tensors*

by means of a *detracing projection operator.* The details are beyond the scope of this study, thus we only describe the traceless $\mathbf{R}^{(n)}$ tensor, using Burnham and English scaling factor, as

$$\mathbf{R}^{t(n)} = (-1)^n \frac{R^{2n+1}}{(2n-1)!!} \boldsymbol{\nabla}^{(n)} \left( \frac{1}{R} \right). \tag{5}$$

This traceless symmetric tensor is referred by Applequist (2002) as *Maxwell-Cartesian spherical harmonics.* For the sake of clarity, we show the first components of this traceless tensor here, where we immediately recognise the dipole, quadrupole, octupole (and higher order) Cartesian polynomials found in more common derivations of multipole expansions

$$R^{t(1)}_{i_1} = R_{i_1}$$

$$R^{t(2)}_{i_1 i_2} = R_{i_1} R_{i_2} - \frac{R^2}{3} \delta_{i_1 i_2}$$

$$R^{t(3)}_{i_1 i_2 i_3} = R_{i_1} R_{i_2} R_{i_3} - \frac{R^2}{5} \left( R_{i_1} \delta_{i_2 i_3} + R_{i_2} \delta_{i_1 i_3} + R_{i_3} \delta_{i_1 i_2} \right)$$

Now we refer to an important observation by Burnham & English (2019) that says if $A^{(n)}$ is a rank $n$ tensor and $B^{t(n)}$ is a traceless tensor of the same rank then the inner product between them satisfies

$$\langle A^{(n)}, B^{t(n)} \rangle_t = \langle A^{t(n)}, B^{t(n)} \rangle_t$$

where $A^{t(n)}$ is the traceless part of $A^{(n)}$.

Using the previous results we can write the magnetic potential of Equation (4)

in terms of the Maxwell-Cartesian spherical harmonic tensor as

$$\Phi(\mathbf{R}) = \gamma_B \sum_{n=0}^{\infty} \frac{(2n-1)!!}{R^{2n+1}} \langle \mathbf{M}^{t(n)}, \mathbf{R}^{t(n)} \rangle_t,$$

where both the multipole tensor and the tensor with the derivatives are traceless symmetric tensors. The components of the traceless multipole tensor can be calculated directly, for example, the quadrupole and octupole tensors read

$$M^{t(2)}_{i_1 i_2} = \frac{1}{2} \int_V \mathrm{d}^3 r \; \lambda(\mathbf{r}) \left[ r_{i_1} r_{i_2} - \frac{r^2}{3} \delta_{i_1 i_2} \right]$$

$$M^{t(3)}_{i_1 i_2 i_3} = \frac{1}{6} \int_V \mathrm{d}^3 r \; \lambda(\mathbf{r}) \left[ r_{i_1} r_{i_2} r_{i_3} - \frac{r^2}{5} \left( r_{i_1} \delta_{i_2 i_3} + r_{i_2} \delta_{i_1 i_3} + r_{i_3} \delta_{i_1 i_2} \right) \right]$$

We remark that the full set of $\mathbf{R}^{t(n)}$ polynomials are not linearly independent because of the vanishing of all the tensor traces. According to this, a minimal linearly independent subset can be specified by suitably taking $2n + 1$ polynomials (Applequist, 2002). Furthermore, these polynomials are not completely orthogonal, in the sense of orthogonality by an inner product in spherical coordinates in the unit sphere (see Section §S8.1). The orthogonality is fully satisfied only for polynomials of different rank index, and partially satisfied by polynomials belonging to tensors of the same rank. Therefore in the following Section we express the tensors in a different basis, namely in the basis of spherical harmonic polynomials, which provide an minimal and completely orthogonal basis.

## S8.1 Spherical harmonic polynomials

Burnham & English (2019) show that symmetric traceless tensors can be described in terms of a minimal set of $2n+1$ linearly independent vectors. They, therefore, use spherical harmonics, which are an orthogonal basis for traceless tensors. An important theorem derived in (Burnham & English, 2019) proves a relation to convert between the inner product of traceless tensors and the spherical inner product of harmonic polynomials, which is defined as

$$\langle u^{(m)}, v^{(n)} \rangle_s = \frac{1}{4\pi} \int_{\Omega} u^{(m)}(\varphi, \theta)\; v^{(n)}(\varphi, \theta)\; \mathrm{d}\Omega,$$

where $u^{(m)}(\varphi, \theta)$ is a real homogeneous polynomial of order $m$ as a function of spherical coordinates, similarly for $v^{(n)}$. Notice that this product is defined using real polynomials thus we do not employ the complex conjugate for $u^{(m)}$. Using the theory of spherical harmonics, Burnham and English employ the spherical harmonic polynomials $q^{i(n)}$, also known as solid harmonics, which are orthogonal over the unit sphere.

From now on we will follow Burnham and English notation for the polynomials (see Burnham & English (2019, p. 14)). However, here we use Greek letters to index the spherical harmonic components, in contrast to Burnham and English notation which uses modern Roman lower case letters.

It is possible to define the *traceless tensor form* of the spherical harmonic polynomials as

$$\mathbf{Q}^{\alpha(n)} = \frac{1}{n!} \boldsymbol{\nabla}^{(n)} q^{\alpha(n)} \tag{6}$$

which satisfy

$$\langle \mathbf{Q}^{\alpha(n)}, \mathbf{Q}^{\beta(n)} \rangle_t = \delta_{\alpha\beta}.$$

The inverse of Equation (6) is computed using the tensor product as (see Burnham & English (2019, p. 17))

$$q^{\alpha(n)}(\mathbf{r}) = \langle \mathbf{Q}^{\alpha(n)}, \mathbf{R}^{i(n)} \rangle_t = \sum_{|n|=n} Q^{\alpha(n)}_{(n_x,n_y,n_z)} R^{(n)}_{(n_x,n_y,n_z)} = \sum_{i_1 i_2 \cdots i_n} Q^{\alpha(n)}_{i_1 i_2 \cdots i_n} R^{(n)}_{i_1 i_2 \cdots i_n},$$

where $n_k$ refers to the number of times the index $k$ occurs in $i_1 i_2 \cdots i_n$, and the sum satisfies $|n| = n_x + n_y + n_z = n$. For instance, the rank-3 spherical harmonic $q^{3(3)}$ given in Table S7 is expressed as a sum of tensor components following

$$\begin{aligned} q^{3(3)} =& \frac{1}{2}\sqrt{\frac{3}{5}} y \left(5z^2 - R^2\right) \\ =& \sqrt{\frac{12}{5}} yz^2 - \sqrt{\frac{3}{20}} x^2 y - \sqrt{\frac{3}{20}} y^3 \\ =& Q^{3(3)}_{yzz} R_{yzz} + Q^{3(3)}_{xxy} R_{xxy} + Q^{3(3)}_{yyy} R_{yyy} \\ =& Q^{3(3)}_{233} R_{233} + Q^{3(3)}_{112} R_{112} + Q^{3(3)}_{222} R_{222} \end{aligned}$$

where we observe that the indices in $Q_{233}$ mean $n_x = 0$, $n_y = 1$ and $n_z = 2$, or $Q_{233} = Q_{(0,1,2)}$. Burnham and English denote the $Q^{\alpha(n)}_{(n_x,n_y,n_z)}$ polynomial coefficients as $\bar{Q}^{\alpha(n)}_{(n_x,n_y,n_z)}$, to distinguish them from the tensor components $Q^{\alpha(n)}_{i_1 \cdots i_n}$.

These definitions of the spherical harmonic polynomials mean that they are normalized as

$$\left\| q^{\alpha(n)} \right\|^2 = \frac{n!}{(2n+1)!!}. \tag{7}$$

| | | | |
|---|---|---|---|
| Degree 1 | $q^{1(1)} = x$ | $q^{2(1)} = y$ | $q^{3(1)} = z$ |
| Degree 2 | $q^{1(2)} = \frac{3z^2-R^2}{\sqrt{6}}$ | $q^{2(2)} = \sqrt{2}xz$ | $q^{3(2)} = \sqrt{2}yz$ |
| | $q^{4(2)} = \frac{\left(x^2-y^2\right)}{\sqrt{2}}$ | $q^{5(2)} = \sqrt{2}xy$ | |
| Degree 3 | $q^{1(3)} = \frac{z\left(5z^2-3R^2\right)}{\sqrt{10}}$ | $q^{2(3)} = \frac{1}{2}\sqrt{\frac{3}{5}}x\left(5z^2 - R^2\right)$ | |
| | $q^{3(3)} = \frac{1}{2}\sqrt{\frac{3}{5}}y\left(5z^2 - R^2\right)$ | $q^{4(3)} = \sqrt{\frac{3}{2}}z\left(x^2 - y^2\right),$ | |
| | $q^{5(3)} = \sqrt{6}xyz$ | $q^{6(3)} = \frac{1}{2}x\left(x^2 - 3y^2\right)$ | |
| | $q^{7(3)} = \frac{1}{2}y\left(3x^2 - y^2\right)$ | | |

SUPP. TABLE S7: Spherical harmonic polynomials derived from real regular spherical harmonics by Stone (2013) and re-normalized by Burnham & English (2019).

Explicit forms of $q^{\alpha(n)}(\mathbf{r})$ are given by Stone (2013, Appendix A and B) based on real regular spherical harmonics and adapted by Burnham & English (2019). We show these polynomials in Table S7. In order to obtain the irregular spherical harmonic polynomials we must divide the polynomials of Table S7 by $R^{2n+1}$.

The $\mathbf{Q}^{\alpha(n)}$ tensor form of the spherical harmonic polynomials provide an orthogonal basis for the traceless symmetric rank $n$ tensors $\mathbf{A}^{(n)}$ such that we can express them as a linear sum in $\mathbf{Q}^{\alpha(n)}$ as

$$\mathbf{A}^{(n)} = \sum_{\alpha=1}^{2n+1} A_\alpha^{(n)} \mathbf{Q}^{\alpha(n)}.$$

By taking the inner product on both sides of this equation we can obtain $A_\alpha^{(n)}$, the components of the $\mathbf{A}^{(n)}$ tensor in the spherical harmonic basis using the usual tensor product

$$A_\alpha^{(n)} = \langle \mathbf{Q}^{\alpha(n)}, \mathbf{A}^{(n)} \rangle_t = \sum_{i_1 i_2 \cdots i_n} Q_{i_1 i_2 \cdots i_n}^{\alpha(n)} A_{i_1 i_2 \cdots i_n}^{(n)}.$$

An important result to obtained from this formalism is that, given the orthogo-

nality of the spherical harmonics, the tensor product of two traceless tensors can be now expressed as a sum of their components in the spherical harmonic basis as

$$\langle \mathbf{A}^{(n)}, \mathbf{B}^{(n)} \rangle_t = \sum_{\alpha=1}^{2n+1} A_\alpha^{(n)} B_\alpha^{(n)}.$$

Additionally, using this property Burnham & English (2019, p. 18) show that the spherical harmonic representation of the Maxwell-Cartesian spherical harmonics are just the spherical harmonic polynomials from Table S7, *i.e.*

$$R_\alpha^{t(n)} = q^{\alpha(n)}(\mathbf{r}).$$

According to this result we can rewrite the multipole expansion tensor product using the spherical harmonic basis as

$$\begin{aligned}\Phi(\mathbf{R}) =& \gamma_B \sum_{n=0}^{\infty} \frac{(2n-1)!!}{R^{2n+1}} \langle \mathbf{M}^{t(n)}, \mathbf{R}^{t(n)} \rangle_t \\ =& \gamma_B \sum_{n=0}^{\infty} \frac{(2n-1)!!}{R^{2n+1}} \sum_{\alpha=1}^{2n+1} M_\alpha^{t(n)} R_\alpha^{t(n)} \\ =& \gamma_B \sum_{n=0}^{\infty} \frac{(2n-1)!!}{R^{2n+1}} \sum_{\alpha=1}^{2n+1} M_\alpha^{t(n)} q^{\alpha(n)}\end{aligned}$$

We must remark that the multipole expansion is now expressed in terms of an orthogonal basis. As a result, it is straightforward to compute the field components as

$$B_i = -\frac{\partial \Phi}{\partial R_i} = \gamma_B \sum_{n=0}^{\infty} \sum_{\alpha=1}^{2n+1} (2n-1)!! M_\alpha^{t(n)} \left( -\frac{\partial Q^{\alpha(n)}}{\partial R_i} \right), \tag{8}$$

with $Q^{\alpha(n)} = R^{-2n-1}q^{\alpha(n)}$. Observe that by dividing $q^{\alpha(n)}$ by $R^{2n+1}$ we have the irregular spherical harmonics defined by Stone (2013).

The expression given by Equation (8) can be further simplified by defining the multipole tensor components as

$$\Theta_{\alpha}^{t(n)} = (2n-1)!!M_{\alpha}^{t(n)},$$

and by defining the multipole polynomials as

$$P_i^{\alpha(n)} = -\frac{\partial Q^{\alpha(n)}}{\partial R_i}.$$

we can write

$$B_i = \gamma_B \sum_{n=0}^{\infty} \sum_{\alpha=1}^{2n+1} \Theta_{\alpha}^{t(n)} P_i^{\alpha(n)}.$$

The multipole polynomials can be easily obtained using Mathematica or the open source library SymPy.

## S8.2 Visualization of harmonics

In order to compare the two different set of basis polynomials describing the $z$-component of the field in the multipole expansion, we computed a graphical representation of the polynomials derived from both the Maxwell-Cartesian harmonics and the polynomials in the spherical harmonic basis. We visualize the polynomials $p(\mathbf{R})$ at the unit sphere ($R = 1$) and using spherical coordinates with the radial component indicating their strength $|p(\mathbf{R})|$ and with a colormap to indicate both

the sign and strength of the functions.

The field components derived from the Maxwell-Cartesian spherical harmonics are obtained by deriving the $\mathbf{R}^{t(n)}$ tensors of Equation (5) as

$$\mathbf{C}_k^{(n)} = -\frac{\partial}{\partial R_k}\left(\frac{\mathbf{R}^{t(n)}}{R^{2n+1}}\right),$$

which decay as $R^{2n+3}$, and such that the $k$-component of the field is written as

$$B_k(\mathbf{R}) = \gamma_B \sum_{n=1}^{\infty} \langle \boldsymbol{\Theta}^{t(n)}, \mathbf{C}^{t(n)} \rangle_t.$$

For example, the quadrupole field polynomials are obtained in the following way

$$\begin{aligned} C_{ij|z}^{(2)} &= -\frac{\partial}{\partial z}\left(R_i R_j - \frac{R^2}{3}\delta_{ij}\right) \\ &= \frac{5R_i R_j R_z - R^2\left(R_i\delta_{jz} + R_j\delta_{iz} + R_z\delta_{ij}\right)}{R^7}. \end{aligned}$$

We observe that the tensor $\mathbf{C}_z^{(2)}$ is traceless. Although these quadrupole polynomials are not orthogonal it is still necessary to find the minimal set of 5 linearly independent elements. By applying the property that the quadrupole tensor is completely symmetric and the fact that the multipole tensor $\boldsymbol{\Theta}^{t(n)}$ is also traceless, we can impose the condition $\Theta_{xx}^{t(2)} + \Theta_{yy}^{t(2)} = -\Theta_{zz}^{t(2)}$ to reduce the 9 polynomials to a set

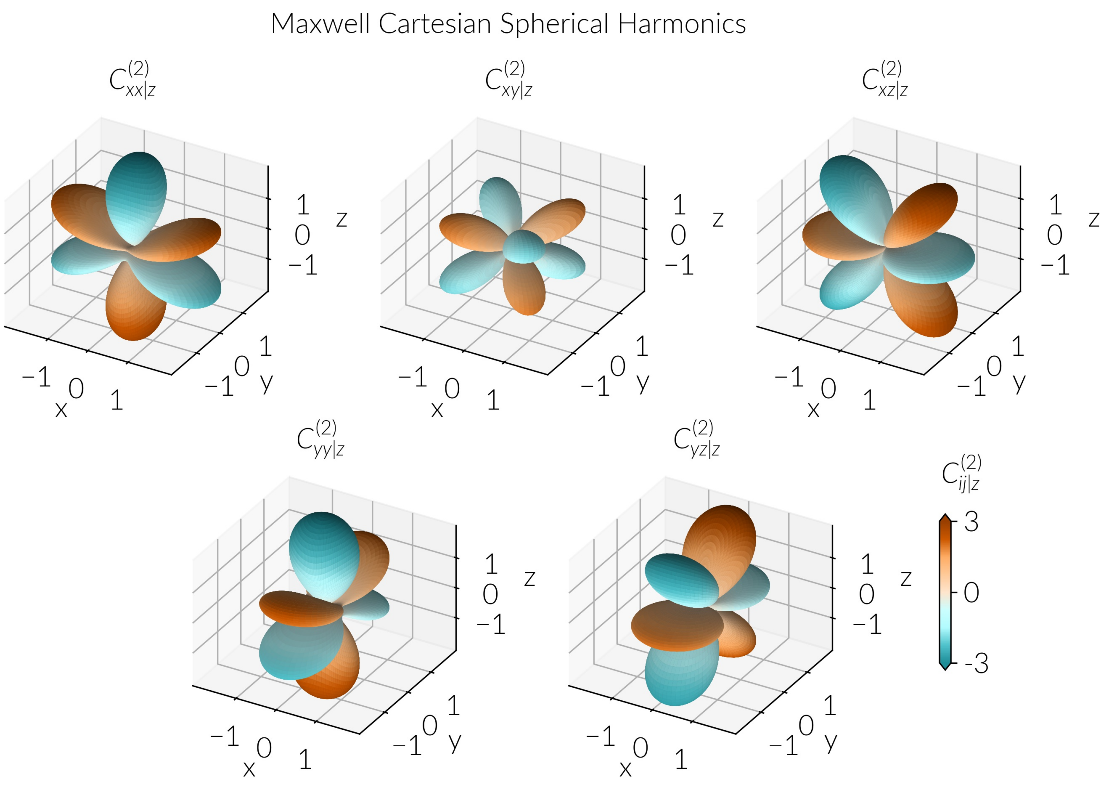


SUPP. FIG. S11: Visual representation of the quadrupole Maxwell-Cartesian harmonic polynomials describing the $z$-component of the magnetic field in the multipole expansion. The harmonics are represented in the unit sphere $R = 1$. The radial distance in the plots indicates the modulus of the polynomials and the colormap indicates both strength and sign of the harmonics.

of 5 terms. If we define $c^{(2)}_{xx|z} = R^7 C^{(2)}_{xx|z}$ we obtain

$$c^{(2)}_{xx|z} = 5z\left(x^2 - z^2\right) + 2R^2 z$$

$$c^{(2)}_{xy|z} = 10xyz$$

$$c^{(2)}_{xz|z} = 2x\left(5z^2 - R^2\right)$$

$$c^{(2)}_{yy|z} = 5z\left(y^2 - z^2\right) + 2R^2 z$$

$$c^{(2)}_{yz|z} = 2y\left(5z^2 - R^2\right)$$

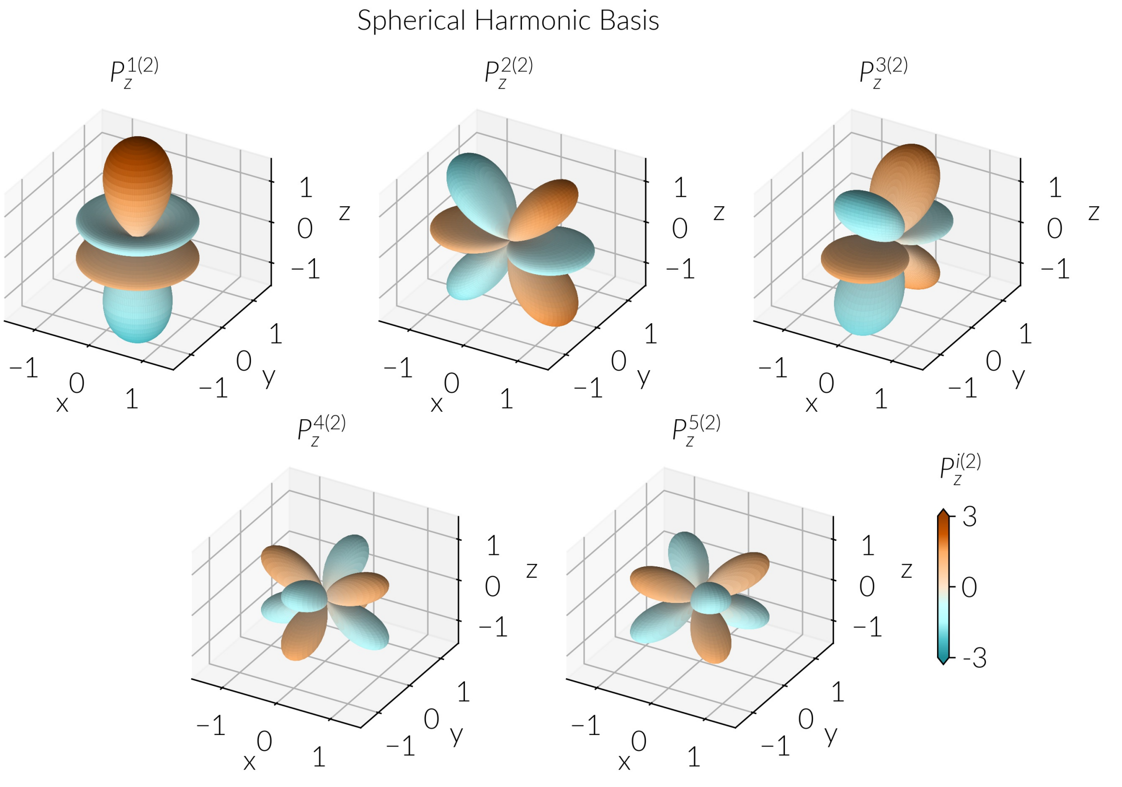


SUPP. FIG. S12: Visual representation of the quadrupole harmonic polynomials in the spherical harmonic basis, describing the $z$-component of the magnetic field in the multipole expansion. The harmonics are represented in the unit sphere $R = 1$. The radial distance in the plots indicates the modulus of the polynomials and the colormap indicates both strength and sign of the harmonics.

These quadrupole polynomials are depicted in Fig. S11. We compare these functions with the case of the polynomials that describe the field components using the spherical harmonics basis, $\mathbf{P}_z^{(2)}$, which we illustrate in Fig. S12. The Maxwell-Cartesian polynomials can be physically interpreted, for example the $C_{xy|z}^{(2)}$ component can be associated with the field generated by two dipoles positioned a distance apart in the $x$ (or $y$) axis and oppositely oriented in the $\pm y$ (or $\pm x$) direction. In contrast, the spherical harmonics are cannot be directly interpreted geometrically in this fashion.

The orientation of the spherical harmonic basis polynomials are clearly different from the Maxwell-Cartesian harmonics. The symmetry of the $P_z^{1(2)}$ function, for instance, is not present in the Maxwell-Cartesian harmonics, although this depends on the chosen set of linearly independent polynomials.

# References


Applequist, J., 2002. Maxwell–Cartesian spherical harmonics in multipole potentials and atomic orbitals, *Theoretical Chemistry Accounts*, **107**(2), 103–115.

Burnham, C. J. & English, N. J., 2019. A New Relatively Simple Approach to Multipole Interactions in Either Spherical Harmonics or Cartesians, Suitable for Implementation into Ewald Sums, *International Journal of Molecular Sciences*, **21**(1), 277.

de Groot, L. V., Fabian, K., Béguin, A., Reith, P., Barnhoorn, A., & Hilgenkamp, H., 2018. Determining individual particle magnetizations in assemblages of micrograins, *Geophys. Res. Lett.*, **45**.

Stone, A., 2013. *The Theory of Intermolecular Forces*, Oxford University Press, Oxford, 2nd edn.
